# Supplementary material for: Effective pruning of web-scale datasets based on complexity of concept clusters
Source: arXiv:2401.04578 source file (2024-03-12)
Supplement: Supplementary file 1 [file qp_appendix.tex]

\section{Quadratic program for Complexity-Based Self-Supervised Prototypes Pruning (CBP)}
\label{app:qp}

In Section ~\ref{sec:CBP}, we introduce CBP where we wish to assess the complexity of data clusters in an embedding space of a pretrained model.
We define the complexity for the j-th cluster $\mathrm{C_j}$ as
\begin{equation}
    \mathrm{C_j}=\mathrm{d_{inter,j}} \cdot \mathrm{d_{intra,j}}.
    \nonumber
\end{equation}
The complexity grows linearly with either \dinter~or \dintra.
Applying a softmax function to $\mathrm{C_j}$ turns it into a probability distribution which we can now sample from.
However, the number of samples per cluster is bounded by the true number of its members.
To honor this bound, we need to solve the following quadratic program: 
\begin{align}
   & \displaystyle{\minimize_{x}}\,\, \frac{1}{2} x^T P x + q^T x  \\
    &  \mathrm{subject\,\,to} \;\;  Ax=b, \; \; l_b \leq x \leq u_b,
    \label{eq:min_x}
\end{align}
where $x$ is the sampled number of examples per cluster, $P$ is the identity matrix and $q=\mathrm{P}_j N$. The first constraint $Ax=b$ bounds the sum of $x$ to the maximum dataset size $N$, so A is a vector of ones and $b=N$. The second constraint bounds $x$ from below by 1 and from above by the true number of items per cluster $N_j$.
Intuitively, the program in Eq.~\ref{eq:min_x} aims to sample $x$ as closely as possible to the probability distribution given by $\mathrm{P}_j$ while honoring the dataset constraints.
We solve the program in Eq.\ref{eq:min_x} with the publicly available quadratic program solver \texttt{qpsolvers} \citep{Caron_qpsolvers_Quadratic_Programming_2023}.
